# Supplementary material for: Role of Structural Morphology in Urban Heat Islands at Night Time
Source: arXiv:1705.00504 ancillary file (2017-05-01)
Supplement: Supplementary file 1 [file SM.pdf]

# Supplemental Material: Role of Structural Morphology in Urban Heat Islands at Night Time

J.M. Sobstyl,[1] T. Emig,[2,3] M.J. Abdolhosseini Qomi,[4] R. J.-M. Pellenq,[1,2,5] and F.-J. Ulm[1,2]

[1] *Concrete Sustainability Hub, Department of Civil and Environmental Engineering, Massachusetts Institute of Technology, Cambridge, Massachusetts, 02139, USA*

[2] *MultiScale Materials Science for Energy and Environment, Joint MIT-CNRS Laboratory (UMI 3466), Massachusetts Institute of Technology, Cambridge, Massachusetts 02139, USA*

[3] *Laboratoire de Physique Theorique et Modeles Statistiques, CNRS UMR 8626, Universite Paris-Saclay, 91405 Orsay cedex, France*

[4] *The Henry Samueli School of Engineering, University of California, Irvine, Irvine, CA 92697*

[5] *Centre Interdisciplinaire des Nanosciences de Marseille, CNRS and Aix-Marseille Universite, Campus de Luminy, Marseille, 13288 Cedex 09, France*

(Dated: April 28, 2017)

In this Supplemental Material, we give details on the approach that we adopted in our work.

### A. Temperature Data

Hourly temperature datasets were obtained from the National Oceanic and Atmospheric Administrations (NOAA) extensive database (Table S1), which is openly available to public users. To minimize the climatic regional difference impact on temperature, we applied the following limiting criteria for selecting weather stations:

- Stations should be within 100km in the horizontal plane.
- Stations should be within 100m in the vertical plane.
- Stations must not be located at major international airports.

For many cities, the above limitations leave more than just a single rural station. To select the most appropriate pair of urban and rural stations, temperatures for those multiple rural stations with the data obtained from the reference urban station are compared. If, for a given day four or less hourly values are missing, they are replaced with daily averages for that day. Days with more than four hourly values missing are disregarded from calculations. Furthermore, a pair of stations must not be used in calculations if file has more than 15% of hourly values missing. If at this point, there is still more than one rural station, the selection is finalized with the pair with the highest UHI. To minimize the error due to high disparity in the signal of temperature variation, UHI was defined as the sum of the nighttime intensity obtained using Fourier transform (Fig. 1) and the median temperature difference (which is closer to the peak of the probability distribution than the mean value). Such defined UHI metric is related to other UHI measuring approaches (i.e. maximum daily, minimum daily, or average daily). In the analysis of temperature data we employed the Fourier transform $\tilde{T}(2\pi/t)$ where $t$ is the time variable of the temperature series. Due to UHI, one would expect that at nighttime cities are on average warmer than areas outside the city, implying that $\Delta T_{u-r} > 0$. In addition, we can conclude that the temperature distribution resembles a periodic signal, which does not change much, since global effects like warming may be neglected for a period of several years. Using the entire distribution of

Temperature and GIS Data

| | | | Urban Station | | | | | Rural Station | | | | |
|---|---|---|---|---|---|---|---|---|---|---|---|---|
| | City | GIS Source | ID | Latitude | Longitude | Start Date | End Date | ID | Latitude | Longitude | Start Date | End Date |
| 1 | Austin, TX | ftp://ftp.ci.austin.tx.us/GIS-Data/Regional/coa_gis.html#environmental | 722544 13958 | +30.321 | -97.760 | 1/1/2006 | 6/30/2015 | 720542 99999 | 30.500 | -97.962 | 8/25/2008 | 6/30/2015 |
| 2 | Boston, MA | MIT University GIS Department | 994971 99999 | +42.350 | -071.050 | 2/1/2010 | 6/30/2015 | 725098 54704 | +42.191 | -071.174 | 1/1/2006 | 6/30/2015 |
| 3 | Chesapeake, VA | https://github.com/jonahadkins/chesapeake-OSM-imports | 997305 99999 | +36.770 | -076.300 | 1/1/2006 | 6/30/2015 | 724007 03719 | +36.682 | -076.602 | 1/1/2006 | 6/30/2015 |
| 4 | Chicago, IL (1) | https://data.cityofchicago.org/Buildings/Building-Footprints/6mpq-sfwi | 997255 99999 | +41.730 | -087.540 | 1/1/2006 | 6/30/2015 | 722059 04866 | +42.690 | -088.304 | 1/1/2006 | 6/30/2015 |
| 5 | Chicago, IL (2) | | 725340 14819 | +41.786 | -087.752 | 1/1/2006 | 6/30/2015 | 722059 04866 | +42.690 | -088.304 | 1/1/2006 | 6/30/2015 |
| 6 | Dallas, TX (1) | http://gis.dallascityhall.com/homepage/shapezip.htm | 722599 03971 | +32.681 | -096.865 | 1/1/2006 | 6/30/2015 | 720287 53967 | 33.714 | -096.674 | 1/1/2006 | 6/30/2015 |
| 7 | Dallas, TX (2) | | 722580 13960 | +32.845 | -096.851 | 8/1/2010 | 6/30/2015 | 720287 53967 | 33.714 | -096.674 | 1/1/2006 | 6/30/2015 |
| 8 | Hartford, CT | https://www.arcgis.com/home/item.html?id=243947f01ac94e0193fff69b2f6b7090 | 725087 14752 | +41.736 | -072.651 | 1/1/2006 | 6/30/2015 | 725098 54704 | +42.191 | -071.174 | 1/1/2006 | 6/30/2015 |
| 9 | Houston, TX (1) | RICE University GIS Department | 720594 00188 | +29.717 | -095.383 | 1/1/2013 | 6/30/2015 | 720926 00313 | +30.071 | -094.216 | 3/10/2011 | 6/30/2015 |
| 10 | Houston, TX (2) | | 998481 99999 | +29.726 | -095.266 | 8/14/2012 | 6/30/2015 | 720926 00313 | +30.071 | -094.216 | 3/10/2011 | 6/30/2015 |
| 11 | Los Angeles, CA (1) | http://egis3.lacounty.gov/dataportal/2011/04/28/countywide-building-outlines/ | 722874 93134 | +34.024 | -118.291 | 1/1/2006 | 6/30/2015 | 722926 03154 | +33.300 | -117.350 | 1/1/2006 | 6/30/2015 |
| 12 | Los Angeles, CA (2) | | 722956 03167 | +33.923 | -118.334 | 1/1/2006 | 6/30/2015 | 722926 03154 | +33.300 | -117.350 | 1/1/2006 | 6/30/2015 |
| 13 | Los Angeles, CA (3) | | 722970 23129 | +33.812 | -118.146 | 1/1/2006 | 6/30/2015 | 722926 03154 | +33.300 | -117.350 | 1/1/2006 | 6/30/2015 |
| 14 | Louisville, KY | http://portal.louisvilleky.gov/dataset/buildings-data | 724235 13810 | +38.228 | -085.664 | 1/1/2006 | 6/30/2015 | 999999 63898 | +38.888 | -086.571 | 10/3/2007 | 6/30/2015 |
| 15 | New York, NY (1) | https://nycopendata.socrata.com/Housing-Development/Building-Footprints/xe92-xce7 | 997272 99999 | +40.639 | -074.146 | 1/1/2006 | 6/30/2015 | 725036 14757 | +41.627 | -073.884 | 1/1/2006 | 6/30/2015 |
| 16 | New York, NY (2) | | 725030 14732 | +40.779 | -073.880 | 1/1/2006 | 6/30/2015 | 725036 14757 | +41.627 | -073.884 | 1/1/2006 | 6/30/2015 |
| 17 | Oklahoma City, OK | https://data.okc.gov/Portal/desktop/page/datasets | 723544 03954 | +35.534 | -097.647 | 1/1/2006 | 6/30/2015 | 720342 53947 | +35.864 | -098.421 | 1/1/2006 | 6/30/2015 |
| 18 | Philadelphia, PA (1) | http://opendataphilly.org/opendata/resource/6/ | 724085 94732 | +40.082 | -075.011 | 1/1/2006 | 6/30/2015 | 720407 99999 | +39.933 | -074.300 | 11/14/2007 | 6/30/2015 |
| 19 | Philadelphia, PA (2) | | 997286 99999 | +39.930 | -075.000 | 1/1/2006 | 6/30/2015 | 720407 99999 | +39.933 | -074.300 | 11/14/2007 | 6/30/2015 |
| 20 | Seattle, WA (1) | https://data.seattle.gov/dataset/2009-Building-Outlines/y7u8-vad7 | 994014 99999 | +47.605 | -122.338 | 1/1/2006 | 6/30/2015 | 727945 04205 | +48.161 | -122.159 | 1/1/2006 | 6/30/2015 |
| 21 | Seattle, WA (2) | | 727934 94248 | +47.493 | -122.214 | 1/1/2006 | 6/30/2015 | 727945 04205 | +48.161 | -122.159 | 1/1/2006 | 6/30/2015 |
| 22 | Washington, DC | http://data.dc.gov/Metadata.aspx?id=59 | 997314 99999 | +38.870 | -077.020 | 7/24/2008 | 6/30/2015 | 723098 93798 | +38.527 | -077.859 | 1/1/2006 | 6/30/2015 |

TABLE I. Temperature datasets from the National Oceanic and Atmospheric Administrations (NOAA) database and Geographical Information System.

temperature differences as the input for calculation, we obtained the spectral distribution to find that the period of 24 hours presenting the highest amplitude, is most exemplary of the signal. Establishing that daily temperature difference coincides with sinusoidal signal allowed us to proceed with analysis of the nighttime $\Delta T_{u-r}$ intensity, which we defined as the sum of Fourier transform and median value of hourly temperature difference, $\Delta\tilde{T}$:

$$\Delta T_{u-r} = \tilde{T}(2\pi/t_{24}) + \Delta\tilde{T}\,. \quad (1)$$

### B. Building Geometric Data

Geographical Information System (GIS) datasets with building footprints were obtained from either university or city GIS departments (Table I). However, the accuracy offered

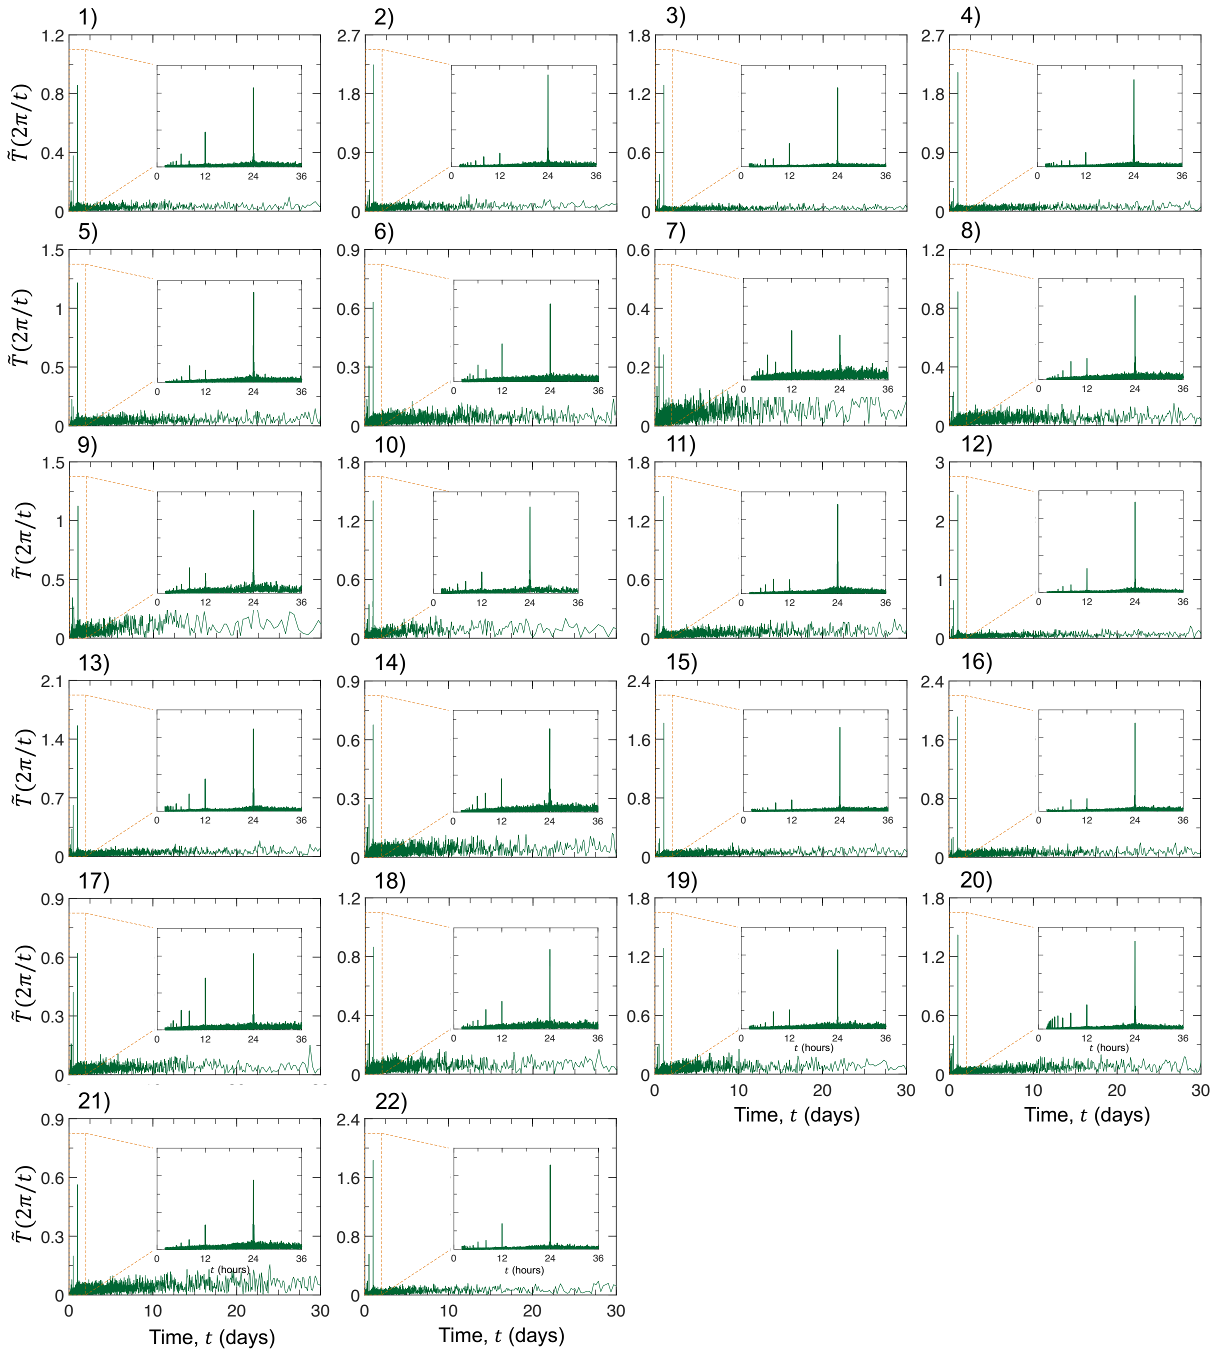


FIG. 1. Fourier transformed times series of urban–rural temperature difference.

by the current online mapping tools suggests that the image classification algorithms for remote sensing could be utilized to extract herein required GIS inputs. For every urban weather station and using 3-mile radius around it, samples of buildings representative of cities were extracted. Such limit, as opposed to other radii, is sufficient to provide statistically significant samples of buildings for proceeding calculations. To focus on the energy

Extracted Urban Geometry and Temperature Data

| | City | $\Delta T_{u-r}$ ($°C$) | $\tilde{T}(2\pi/t_{24})$ | $R$ ($m$) | $L$ ($m$) | $d$ ($m$) |
|---|---|---|---|---|---|---|
| 1 | Austin, TX | 1.8 | 0.9 | 26.8 | 14.5 | 18.1 |
| 2 | Boston, MA | 2.7 | 2.2 | 21.6 | 11.3 | 14.7 |
| 3 | Chesapeake, VA | 1.7 | 1.3 | 35.9 | 12.1 | 24.6 |
| 4 | Chicago, IL (1) | 4.2 | 2.1 | 17.0 | 11.3 | 9.9 |
| 5 | Chicago, IL (2) | 3.5 | 1.2 | 16.6 | 10.9 | 9.5 |
| 6 | Dallas, TX (1) | 1.9 | 0.6 | 32.5 | 14.5 | 19.9 |
| 7 | Dallas, TX (2) | 1.9 | 0.2 | 27.1 | 14.6 | 18.3 |
| 8 | Hartford, CT | 2.6 | 0.9 | 25.5 | 11.8 | 15.6 |
| 9 | Houston, TX (1) | 2.1 | 1.1 | 25.9 | 12.1 | 17.0 |
| 10 | Houston, TX (2) | 2.7 | 1.4 | 25.7 | 11.5 | 17.0 |
| 11 | Los Angeles, CA (1) | 3.1 | 1.4 | 21.2 | 13.4 | 14.8 |
| 12 | Los Angeles, CA (2) | 2.9 | 2.4 | 21.9 | 13.0 | 16.0 |
| 13 | Los Angeles, CA (3) | 2.8 | 1.6 | 25.5 | 13.2 | 16.5 |
| 14 | Louisville, KY | 2.8 | 0.7 | 27.1 | 12.6 | 18.2 |
| 15 | New York, NY (1) | 3.8 | 1.8 | 20.4 | 10.8 | 13.1 |
| 16 | New York, NY (2) | 4.2 | 2.3 | 17.8 | 12.5 | 8.3 |
| 17 | Oklahoma City, OK | 1.4 | 0.6 | 30.9 | 15.8 | 21.3 |
| 18 | Philadelphia, PA (1) | 2.0 | 0.9 | 26.8 | 12.5 | 18.1 |
| 19 | Philadelphia, PA (2) | 3.0 | 1.3 | 21.1 | 13.9 | 15.8 |
| 20 | Seattle, WA (1) | 2.9 | 1.4 | 21.7 | 12.4 | 14.1 |
| 21 | Seattle, WA (2) | 2.0 | 0.6 | 27.8 | 12.6 | 18.3 |
| 22 | Washington, DC | 2.7 | 1.8 | 21.6 | 13.5 | 15.9 |

TABLE II. Measured temperature and geometric data for the 22 cities of group A.

transfer between separated buildings or blocks, we merged all buildings sharing the same wall. We analyzed areas of merged buildings and found that in a logarithmic mode probability distribution function of buildings areas can be adequately captured with a bi-modal fit (Fig. 2), which forms a clear distinction between unoccupied and occupied buildings, for instance garages and residential or commercial units, respectively. Unoccupied buildings are disregarded under the assumption that their contribution to the energy transfer between buildings is negligible, while the occupied buildings are represented by their two-dimensional center of mass.

### C. Radial Distribution Function, $g(r)$

We used the two-dimensional center of mass points of the buildings as input values for the calculation of radial distribution function $g(r)$, defined as:

$$g(r) = \frac{1}{N}\sum_{i=1}^{N}\frac{n_i(r+dr)-n_i(r)}{\bar{\rho}_{city}2\pi r dr}\,, \tag{2}$$

where $n_i(r)$ denotes the number of buildings within the radial distance $r$ from building $i$, $dr$ is an "infinitesimal" distance , which we chose to be 5% of the average building size $L$; average building density, $\bar{\rho} = N/A_{ground}$, where $N$ is the total number of buildings inside a box of area, $A_{ground}$, which is defined by a square of length $10L$. We use smaller than area of the city box for in order to be able to obtain the convergence towards unity for the radial distribution function. Since the area of the entire city includes large areas with no buildings present, such as parks and water surfaces, its normalization underestimates the average density, subsequently leading to overestimated values of $g(r)$. Since the distribution of occupied buildings resembles a log-normal form, with the median value capturing its peak, under the assumption that footprints of buildings are of uniform shape (i.e. square) we chose to define the average building size, $L$, as:

$$L = \exp\left[\frac{1}{2N}\sum_{i=1}^{N}\log A_{b_i}\right]\,, \tag{3}$$

where $A_{b_i}$ is the ground area of building $i$.

### D. Heat Radiation Model

We employed a scaling approach to model the dependence of the urban–rural temperature difference $\Delta T_{u-r}$ on urban morphology, described by the characteristic length scales of $g(r)$. We denote the average temperature of flat urban surfaces by $T_{\mathrm{u,flat}}$ and the usually different average temperature of flat rural surfaces by $T_r$. The difference between this two temperatures is due to material and climate induced processes, which are summarized in the relation $T_{\mathrm{u,flat}} = \gamma T_r$ with a phenomenological coefficient $\gamma$. Please note that this relation applies to flat surfaces and does not account for urban geometry, i.e., the size, height and shape of buildings and their separation. The coefficient $\gamma$ hence depends on the difference between thermal admittance and evapotranspiration properties in the rural and urban areas. To describe the effect of urban morphology, we resort to the device of an effective

temperature that is often used for a body as an estimate of its surface temperature when the emissivity is not known [1]. The effective temperature $T_{\rm eff}$, defined as the temperature of a black body with the same power $P$ radiated as the original body so that, according to the Stefan-Boltzmann law, $P = \sigma A T_{\rm eff}^4$ where $A$ is the surface area of the body and $\sigma$ is the Stefan-Boltzmann constant. The urban structure of city can be considered as a rough surface on the length scale of buildings with its effective emissivity not known. We expect that the effective temperature for the IR heat radiation of an urban structure is mainly determined by the increase in its surface area due to building surfaces (assuming that multiple reflections of heat radiation between surfaces can be neglected). Following the above definition of an effective temperature, the effective urban temperature $T_u$ is given by the relation $A_{\rm ground} T_u^4 = A_{\rm actual} T_{\rm u,flat}^4$ where $A_{\rm ground}$ is surface area of the ground covered by the urban structure and $A_{\rm actual}$ its actual surface area including buildings surfaces like walls and roofs. The scaling of the surface area ratio $A_{\rm actual} = A_{\rm ground}$ can be estimated from the typical distance $d$ between buildings, and their mean linear size $L$ and mean height $\bar{h}$. The building wall area is approximately $4L\bar{h}$ and the number of buildings scaling as $A_{\rm ground}/(d+L)^2$ where $(d+L)^2$ is the typical area of an elementary urban block consisting of a building and the adjacent open space. Hence the actual urban surface area becomes

$$A_{\rm actual} = \left[1 + \frac{4L\bar{h}}{(L+d)^2}\right] A_{\rm ground} \equiv \delta(L, \bar{h}, d) A_{\rm ground} \, , \tag{4}$$

so that the effective urban temperature scales as $T_u = T_{\rm u,flat}\delta^{1/4}$ and the amplitude of the UHI, i.e., the rural–urban temperature difference is given by

$$\Delta T_{u-r} = T_u - T_r = T_r(\gamma\delta^{1/4} - 1) \, . \tag{5}$$

### E. Urban Surface Temperature from Solar Radiance

The surface temperature $T_r = T_{\rm u,flat}$ obtained from the fit of Eq. (1) in the main text with $\gamma = 1$ to the data shown in Fig. 3 (main text) can be estimated from a simple radiation balance model. A flat surface is characterized by an emissivity $\epsilon$, a thickness $s$, and thermal conductivity $\kappa$. On the inside of the surface an equilibrium temperature is maintained. Assuming that the surface receives a homogeneous solar radiant flux $L_0$ from the outside, we can estimate the equilibrium temperatures $T_{\rm out}$ on the outside of the surfaces by equating the internal and external net flux densities. The internal net flux is obtained from the stationary

heat conduction equation $q_{\rm int} = -\kappa \partial_n T$ integrated across the surface thickness $s$ yielding $q_{\rm int} = (T_{\rm out} - T_{\rm int})\kappa/s$. The external net flux $q_{\rm ext}$ is obtained as the sum of the incoming solar flux $L_0$ and the heat flux $\epsilon\sigma T_{\rm out}^4$ radiated by the surface where $\sigma$ is the Stefan-Boltzmann constant. The condition $q_{\rm ext} = q_{\rm int}$ then yields

$$(T_{\rm out} - T_{\rm int})\kappa/s = \epsilon(L_0 - \sigma T_{\rm out}^4)\,, \tag{6}$$

which determines the outside surface temperature $T_{\rm out}$ of the surface that can be identified with $T_r$. The result $T_r = 24.4°$C obtained from the fit to our model is reproduced by the typical parameters $\epsilon = 0.92, \kappa = 1$W/mK, $s = 20$cm for an interior building temperature of $T_{\rm int} = 22°$C and a solar radiance of $L_0 = 458$W/m$^2$.

---

[1] A. E. Roy and D. Clarke, *Astronomy: principles and practice*, 4th ed. (Institute of Physics Pub, Bristol ; Philadelphia, 2003).

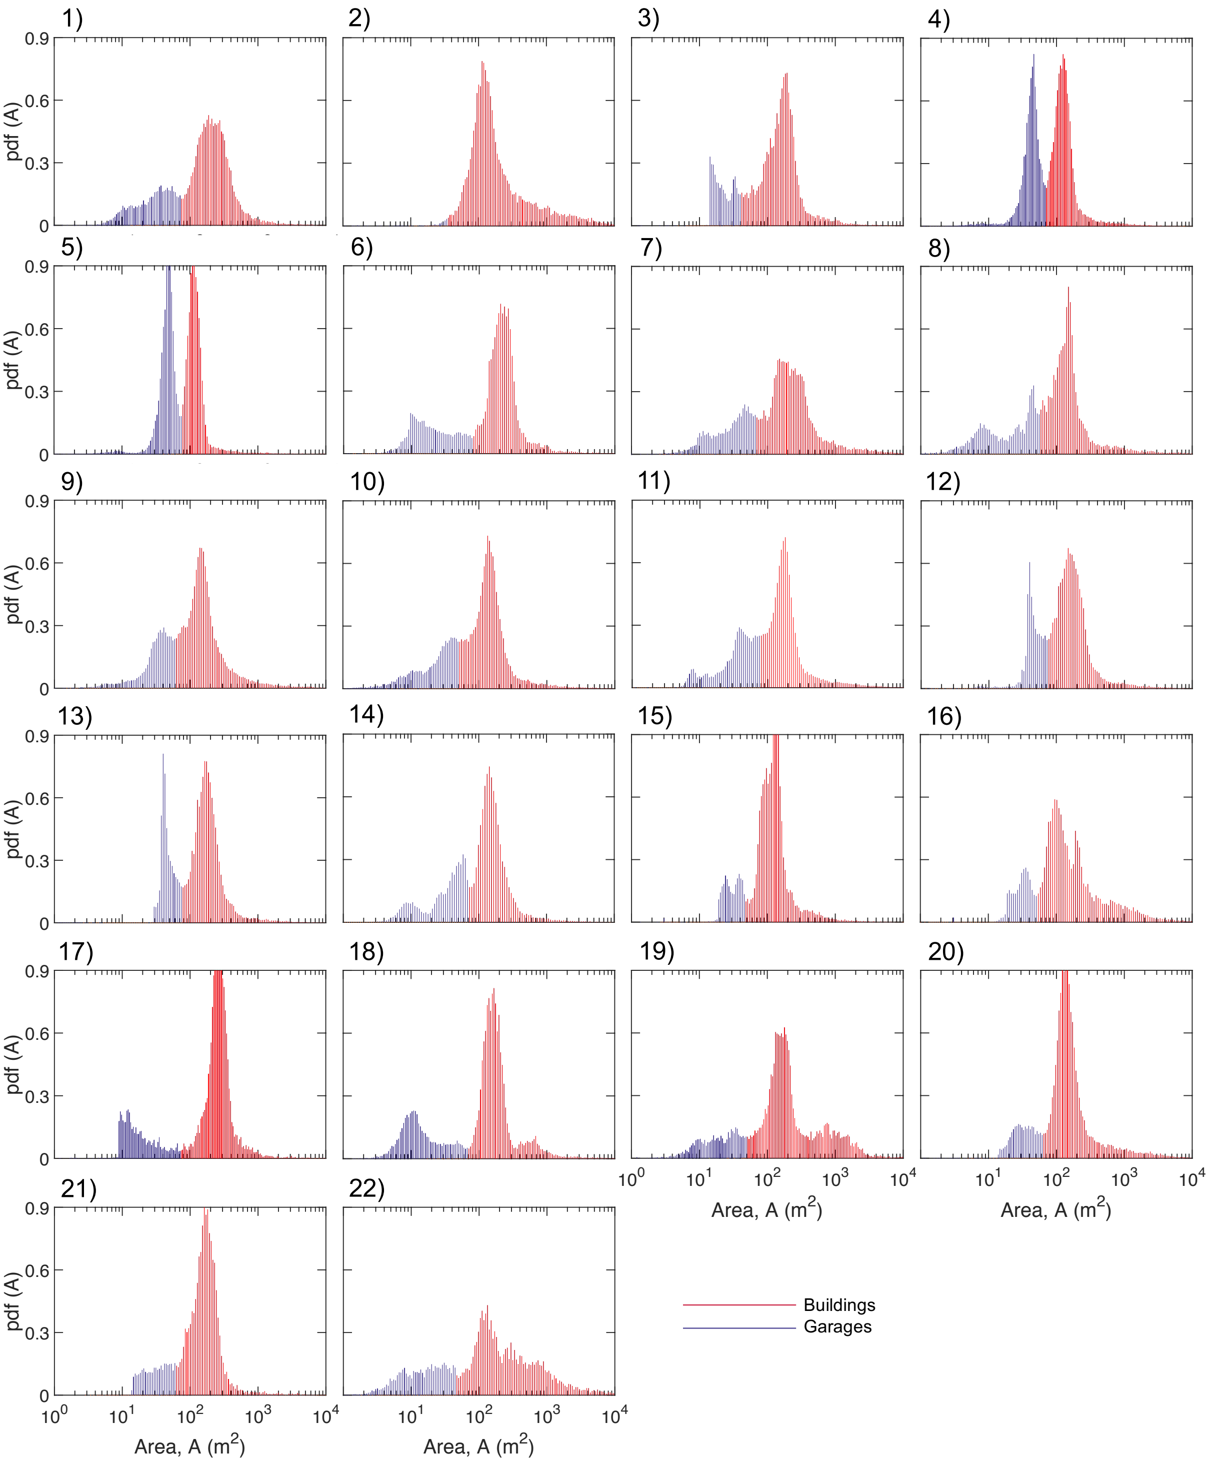


FIG. 2. Probability distribution function of buildings areas.

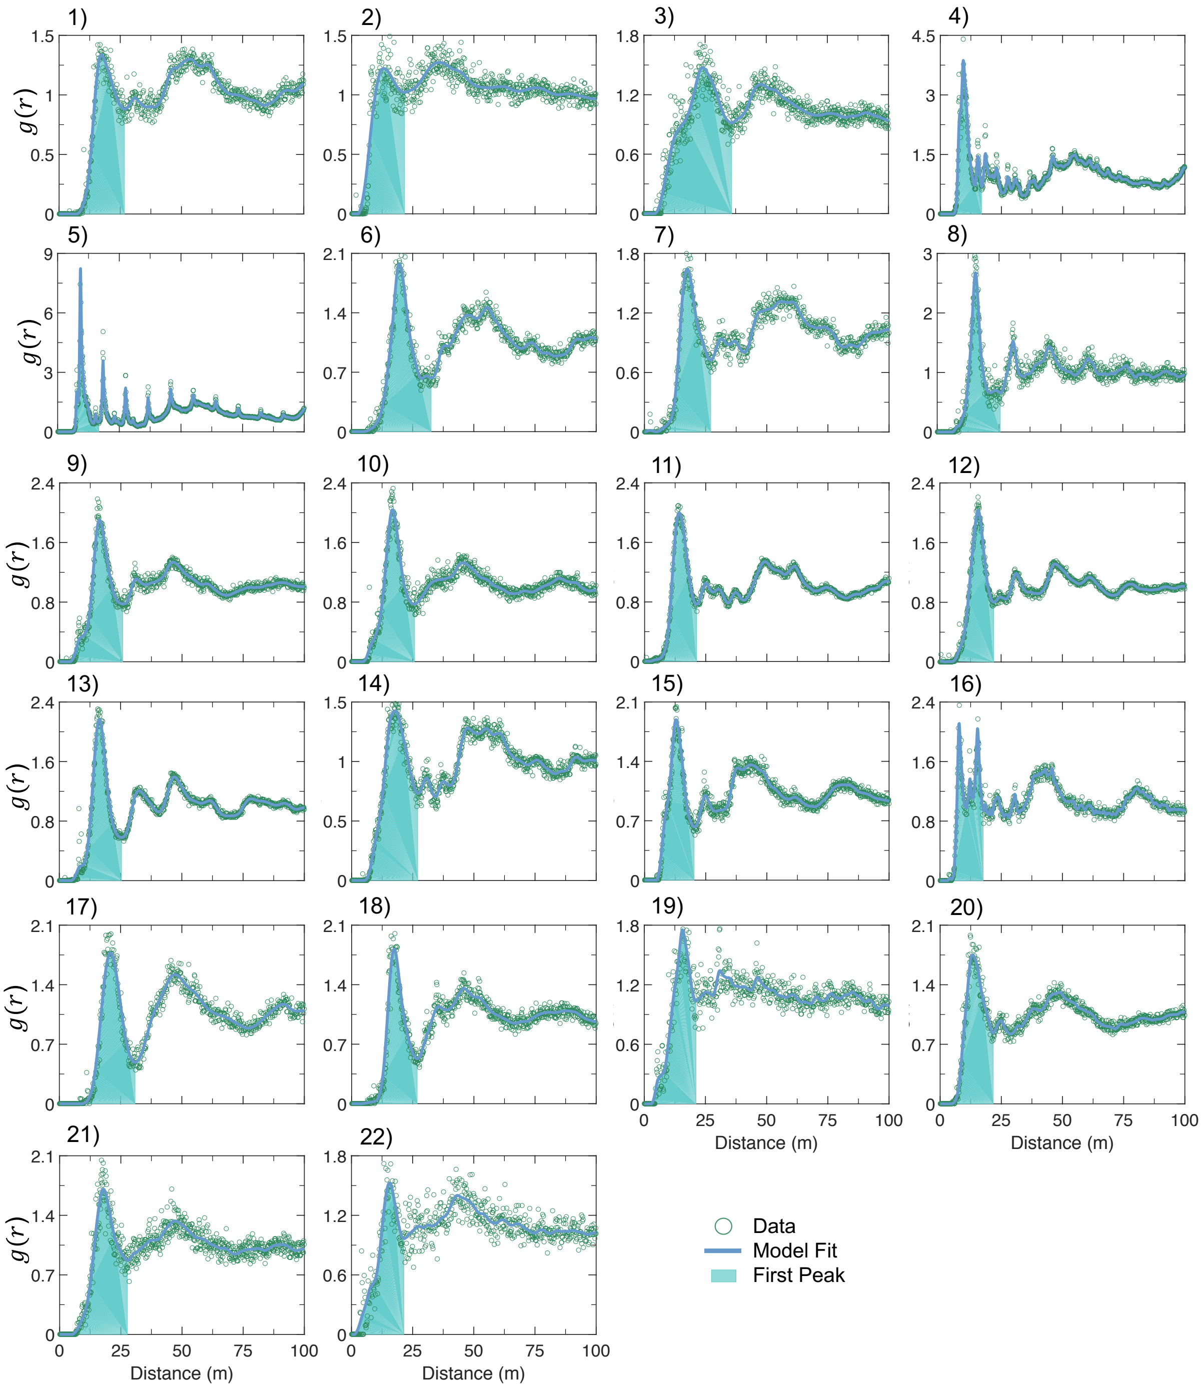


FIG. 3. Radial distribution functions for the 22 cities of group A.
